# Supplementary material for: aiXamine: Simplified LLM Safety and Security
Source: arXiv:2504.14985 source file (2025-04-23)
Supplement: Supplementary file 1 [file 10.appendices.tex]

\appendix
